# Supplementary material for: Quantifying Confidence in DFT Predicted Surface Pourbaix Diagrams of Transition Metal Electrode-Electrolyte Interfaces
Source: arXiv:1710.08407 source file (2018-07-05)
Supplement: Supplementary file 1 [file Pourbaix_SI.pdf]

# Supporting Information: Quantifying Confidence in DFT Predicted Surface Pourbaix Diagrams of Transition Metal Electrode-Electrolyte Interfaces

Olga Vinogradova,† Dilip Krishnamurthy,‡ Vikram Pande,‡ and Venkatasubramanian Viswanathan*,‡,†

†*Department of Chemical Engineering, Carnegie Mellon University, Pittsburgh, PA 15213, USA*

‡*Department of Mechanical Engineering, Carnegie Mellon University, Pittsburgh, PA 15213, USA*

## 1 Calculation Details

All calculations were performed using the projector augmented-wave (PAW)[1,2] method as implemented in GPAW[3,4] with the ASE interface[5]. The Bayesian Error Estimation Functional with Van der Waals corrections (BEEF-vdW)[6] exchange-correlation functional was employed, which has built-in error estimation capabilities and is calibrated to reproduce the error as mapped to experimental training data. This error estimation capability has been used to quantify uncertainty in heterogenous catalysis[7], electrocatalytic actiivty[8,9], magnetic ground states[10] and mechanical properties of solid electrolytes[11].

For (111) facet surfaces, $OH^*$ adsorption is modeled on a $(\sqrt{3} \times \sqrt{3})R30^\circ$ unit cell and

$O^*$ is modeled on a (2×2) unit cell each consisting of 4 layers of metal atoms. The k-point grids are 4×4×1 and 6×6×1 respectively. For (100) facet, 4 layer unit cells of (2×2) and (2×3) were used with 4×4×1 and 6×4×1 k-point grids. A real space grid discretization of 0.18Å was used for all calculations. All DFT calculations were converged with respect to k-point and grid spacing. Each unit cell was periodic in the x and y directions only with 5Å layer of vacuum in z direction above and below the layers. The bottom two layers were fixed and the top two layers including any adsorbates were relaxed to a net force less than 0.05eV/Å. A Fermi smearing of 0.05 eV was used to ensure self consistency in calculation of electron occupations.

## 2 Lattice Parameters

The lattice sizes for each metal were extracted from bulk optimized crystal structures using the BEEF-vdW exchange-correlation functional. The a lattice parameters used in all subsequent simulations are 4.022 Å for Pt, 4.015 Å for Pd, 3.897 Å for Ir Å 3.890 Å for Rh, and 2.738 Å and 4.332 Å for a and c respectively for Ru.

## 3 Calculating Adsorption Energies

The adsorption energies of these intermediates calculated using the BEEF-vdW best-fit functional are reported in Table S1. The standard deviations of all adsorbed surface states are also reported as $\sigma_{O^*}$ or $\sigma_{OH^*}$ as the fraction of BEEF-vdW ensemble functionals in agreement with the best-fit functional.

Table S1: Adsorption Energies of the various intermediates considered on the surface of transition metal surfaces. All energies are reported in eV. All O* intermediates adsorbed at the hollow site unless italicized, which signal intermediates that relaxed to the bridge site. All errors are reported as the standard deviation of the BEEF ensemble.

| | Pt(111) | Pt(100) | Pd(111) | Ir(111) | Rh(111) | Ru(0001) |
|---|---|---|---|---|---|---|
| 1/3 OH $H_2O$ | 0.68 ± 0.23 | 0.65 ± 0.32 | 0.69 ± 0.32 | 0.21 ± 0.23 | 0.20 ± 0.30 | -0.30 ± 0.27 |
| 1/2 OH $H_2O$ | - | 0.73 ± 0.30 | - | - | - | - |
| 1/4 O | 0.64 ± 0.11 | 0.92 ± 0.13 | 0.65 ± 0.14 | 0.40 ± 0.10 | 0.34 ± 0.13 | 0.07 ± 0.08 |
| 1/3 O | 0.92 ± 0.09 | *1.22 ± 0.12* | 0.67 ± 0.13 | 0.39 ± 0.05 | 0.40 ± 0.11 | -0.02± 0.08 |
| 1/2 O | 0.78 ± 0.12 | *0.79 ± 0.17* | 0.79 ± 0.14 | 0.47 ± 0.05 | 0.47 ± 0.13 | 0.11 ± 0.11 |
| 2/3 O | 0.88 ± 0.11 | *1.27 ± 0.13* | 0.91 ± 0.13 | 0.54 ± 0.06 | 0.55 ± 0.11 | 0.11 ± 0.09 |
| 3/4 O | 0.97 ± 0.11 | *0.87 ± 0.13* | 0.97 ± 0.13 | 0.60 ± 0.07 | 0.58 ± 0.13 | 0.18 ± 0.10 |
| 1 O | 1.13 ± 0.11 | 1.35 ± 0.10 | 1.17 ± 0.12 | 0.75 ± 0.07 | 0.70 ± 0.12 | 0.25 ± 0.10 |

# 4 Adsorption on Bulk Oxide Slabs

The OH* intermediate was absorbed at the cus sites of 4 layer rutile (110) metal-oxide slabs where the bottom two layers are constrained. The following figure shows the structure for any metal-oxides considered.

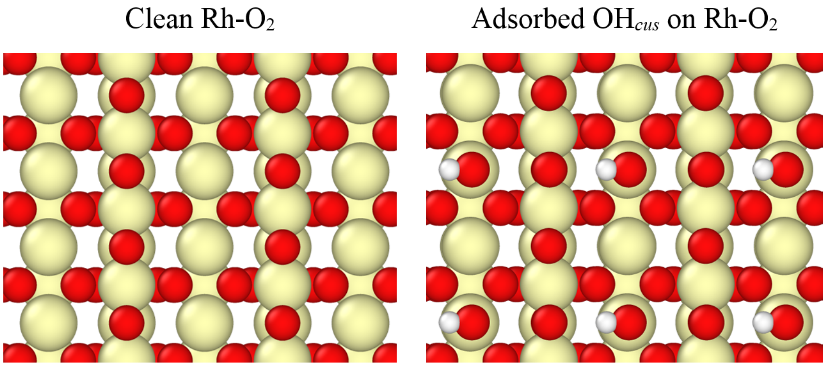


Figure S1: Structure of clean and OH* adsorbed surface for $RhO_2$.

The adsorption energy is calculated by the following equation consistent with the generalized form in the main paper:

$$\Delta E_{OH*} = E_{OH*} - E_{*} - E_{H_2O} + 1/2 E_{H_2} \quad (1)$$

# 5 Zero Point and Entropy Corrections

We report the $\Delta ZPE$ and $\Delta S^{\circ}$ for all reactions at standard temperature T=298 K in Table S2.[12,13]

Table S2: Zero point and entropic corrections to the free energies

| | TS | TΔS | ZPE | ΔZPE | $\Delta ZPE - T\Delta S$ |
|---|---|---|---|---|---|
| $H_2O$ | 0.67 | 0 | 0.56 | 0 | 0 |
| $OH^* + \frac{1}{2}H_2$ | 0.20 | -0.47 | 0.44 | -0.12 | 0.35 |
| $O * + H_2$ | 0.41 | -0.27 | 0.34 | -0.22 | 0.05 |
| $\frac{1}{2}O_2 + H_2$ | 0.73 | 0.05 | 0.32 | -0.24 | -0.29 |
| $H_2$ | 0.41 | | 0.27 | | |
| $\frac{1}{2}O_2$ | 0.32 | | 0.05 | | |
| $O^*$ | 0 | | 0.07 | | |
| $OH^*$ | 0 | | 0.30 | | |
| $H^*$ | 0 | | 0.17 | | |

# 6 Quantifying Confidence in Adsorption Energies

Using the BEEF-vdW best-fit functional, the ensemble of adsorption energies for each surface phase were calculated. The energies were referenced to a clean Pt(111) surfaces since the error is much smaller due to similarities in metal-adsorbate bonding characteristics. We calculate the error of each adsorption energy as the standard deviation of the ensemble spread of energies. The errors are tabulated in table S1. Smaller errors imply similarity in surface-adsorbate interactions of metal surfaces.

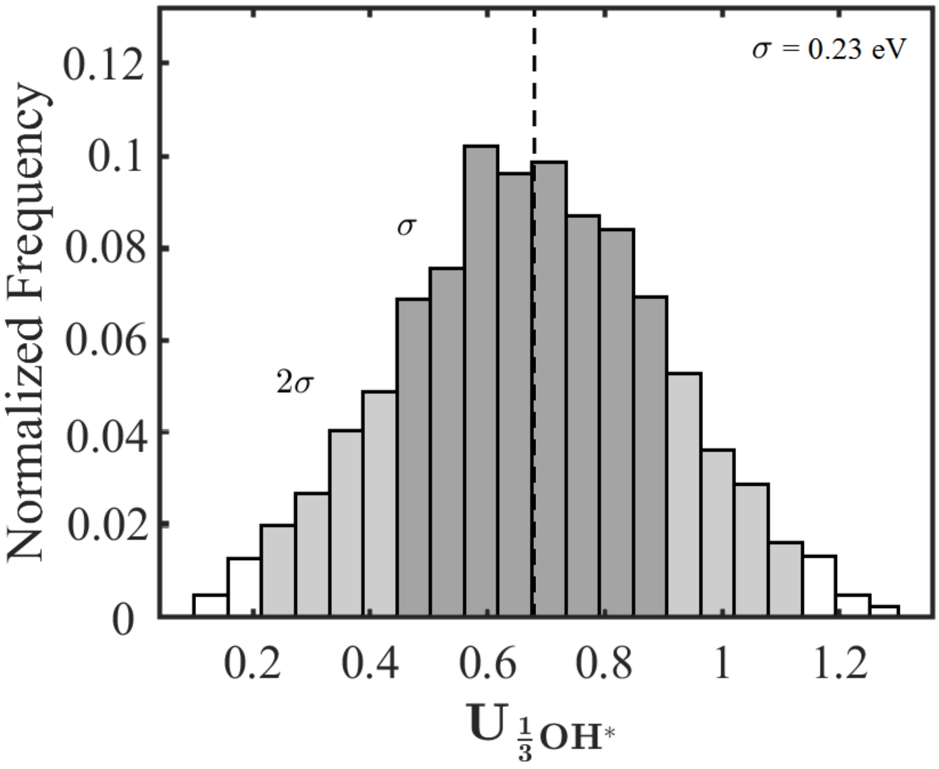


Figure S2: Normalized frequency as a function of adsorption energy of 1/3 $OH^*$ on Pt(111) metal surface. The standard deviation of the spread of energies is $\sigma_{OH}$=0.23 eV.

# 7 Free Energy Ensemble for Pt(111) Surface

To illustrate the ensemble of energies derived from the BEEF-vdW ensemble of functionals, in figure 2 in the main paper we reported a consistent set of 50 energies bounding each of the energies calculated using the best-fit functional. The following figures show the ensemble spread of energies around each individual solution derived with the best-fit functional. All surface state energies are reported in reference to a clean Pt(111) surface.

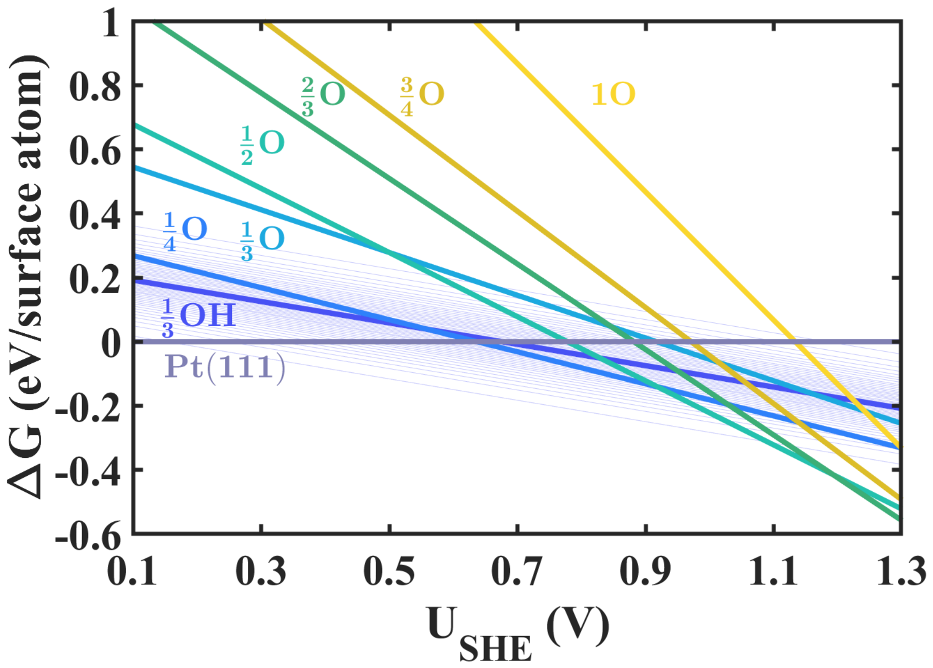


Figure S3: Distribution of energies derived from 50 BEEF-vdW ensemble functionals about the 1/3 $OH^*$ surface phase.

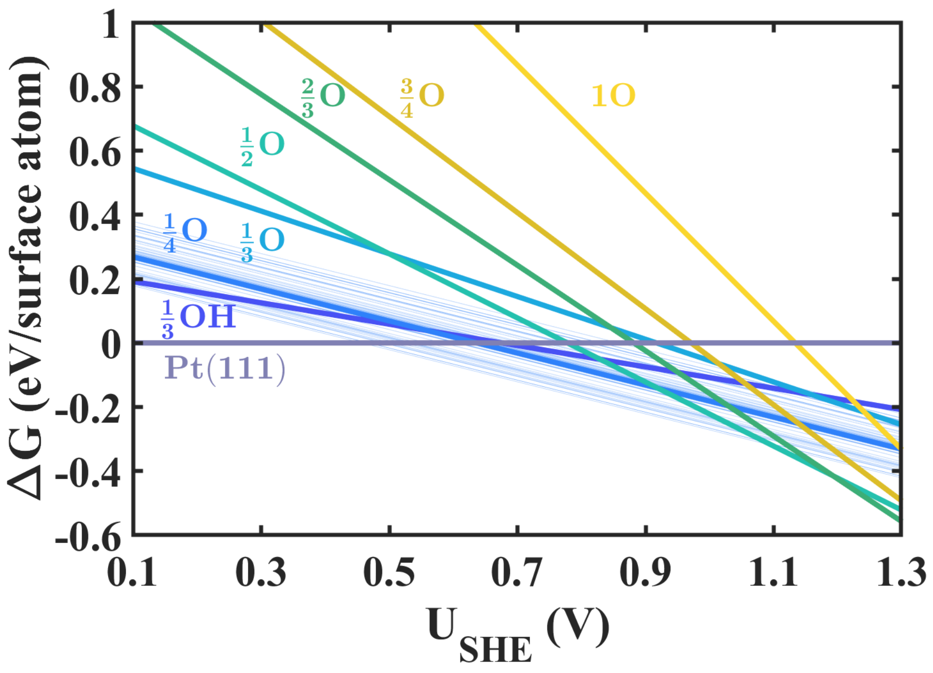


Figure S4: Distribution of energies derived from 50 BEEF-vdW ensemble functionals about the 1/4 O* surface phase.

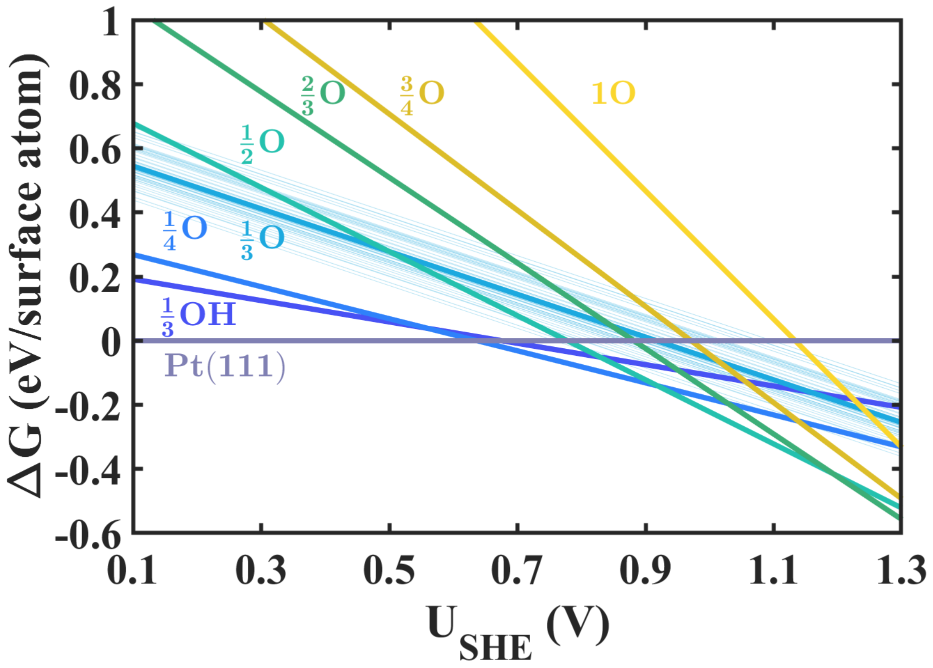


Figure S5: Distribution of energies derived from 50 BEEF-vdW ensemble functionals about the 1/3 O* surface phase.

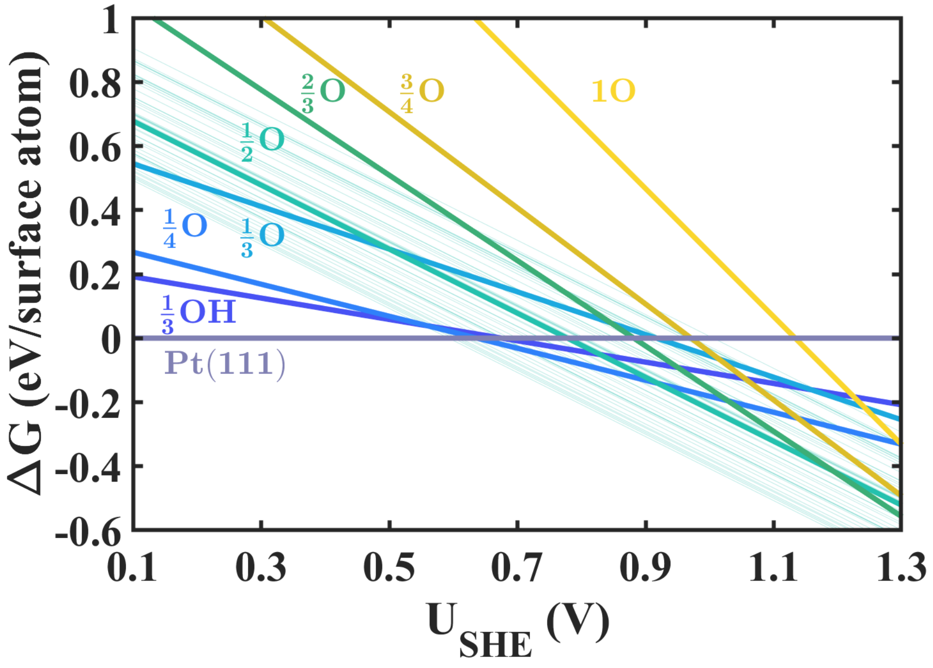


Figure S6: Distribution of energies derived from 50 BEEF-vdW ensemble functionals about the 1/2 O* surface phase.

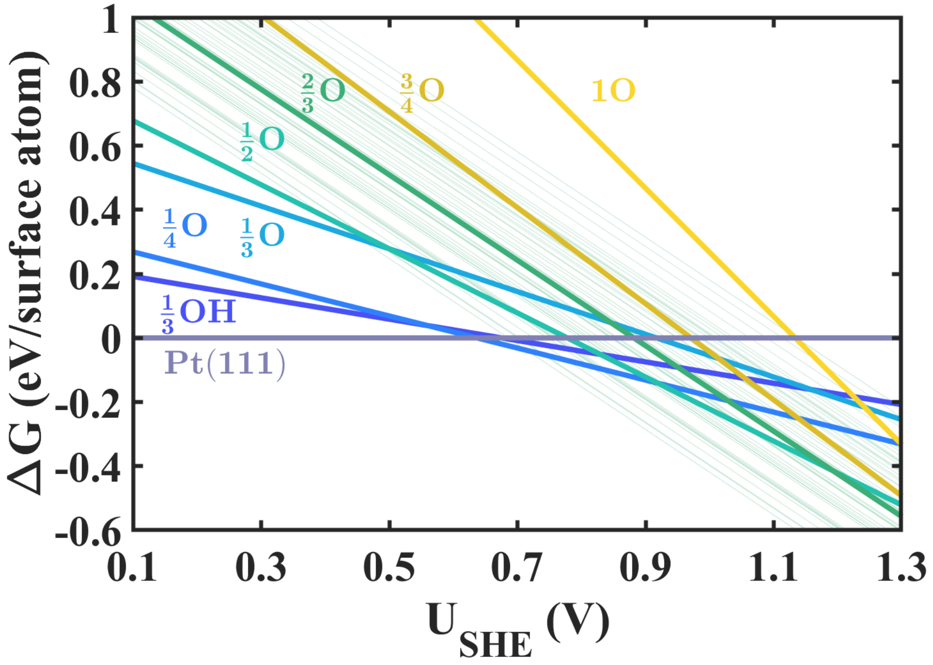


Figure S7: Distribution of energies derived from 50 BEEF-vdW ensemble functionals about the 2/3 O* surface phase.

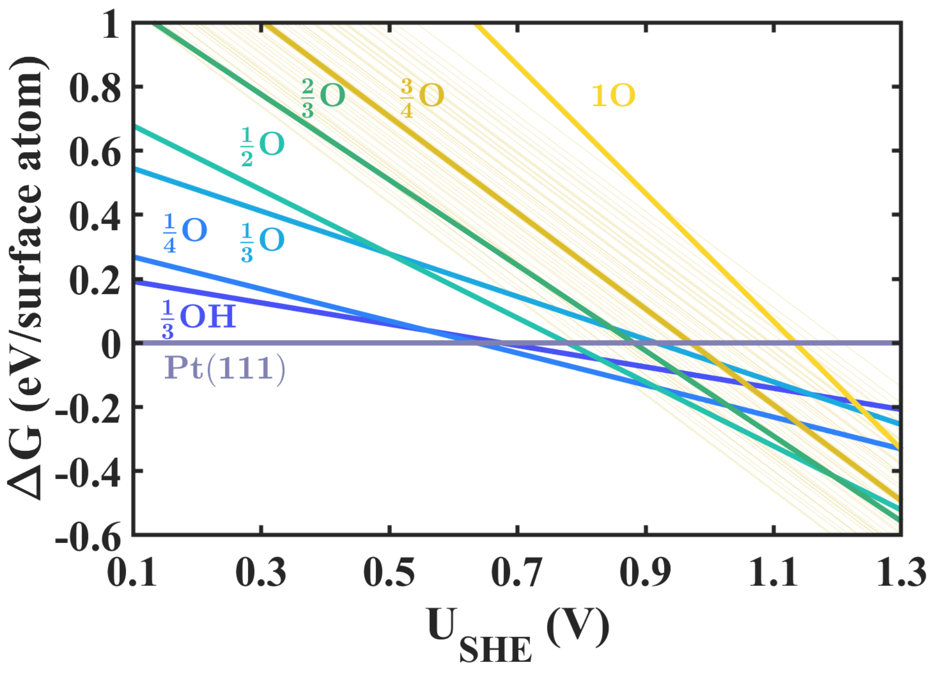


Figure S8: Distribution of energies derived from 50 BEEF-vdW ensemble functionals about the 3/4 O* surface phase.

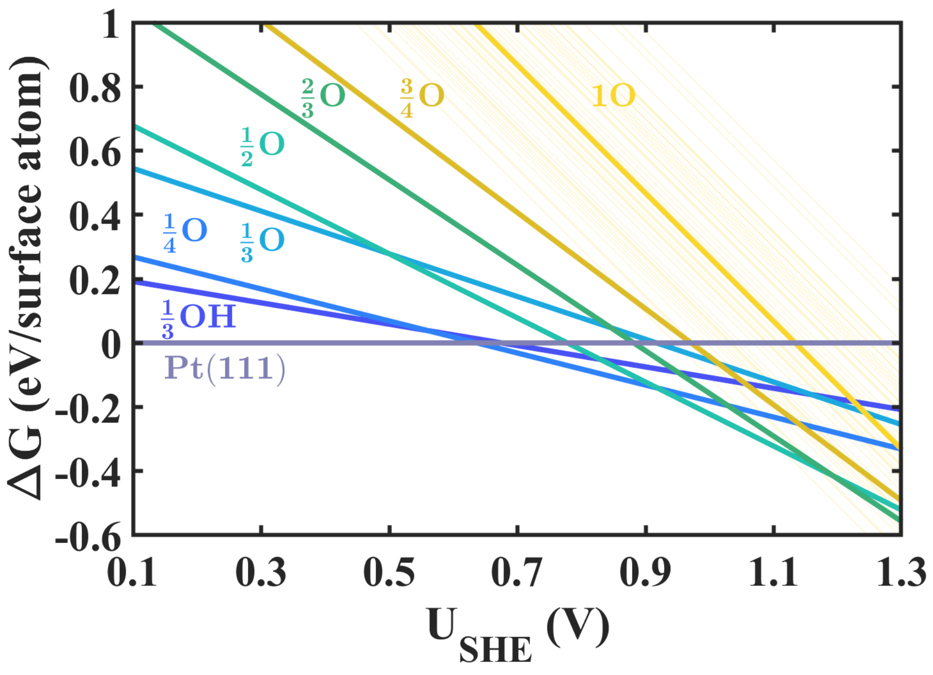


Figure S9: Distribution of energies derived from 50 BEEF-vdW ensemble functionals about the 1 O* surface phase.

# 8 Prediction Confidence at Nonzero pH Levels

In section 3.1 of the main paper, we presented figure 3b showing the prediction confidence of each surface state at a pH of 0. Here, we show that we can extend the prediction confidence of each surface state to other pH values by shifting the x axis by -59 mV/pH. To demonstrate this analysis, we show prediction confidence for each surface phase examined for Pt(111) surface in figure S11 at pH of 7. At $U_{SHE}$ of approximately 0.2 V, we observe a region of low confidence (c-value<0.4) where the surface may be either 1/3 OH*, 1/4 O*, or clean Pt(111). The 1/4 O* surface shows high confidence (≈0.6) at about 0.4 V which transitions to the 1/2 O* surface at ≈0.4 V and to the 2/3 O* surface phase at ≈0.8 V before the dissolution potential of 1.18 V for Pt(111). We highlight that this shows the necessity of utilizing the prediction confidence metric to more accurately describe surface phase transitions.

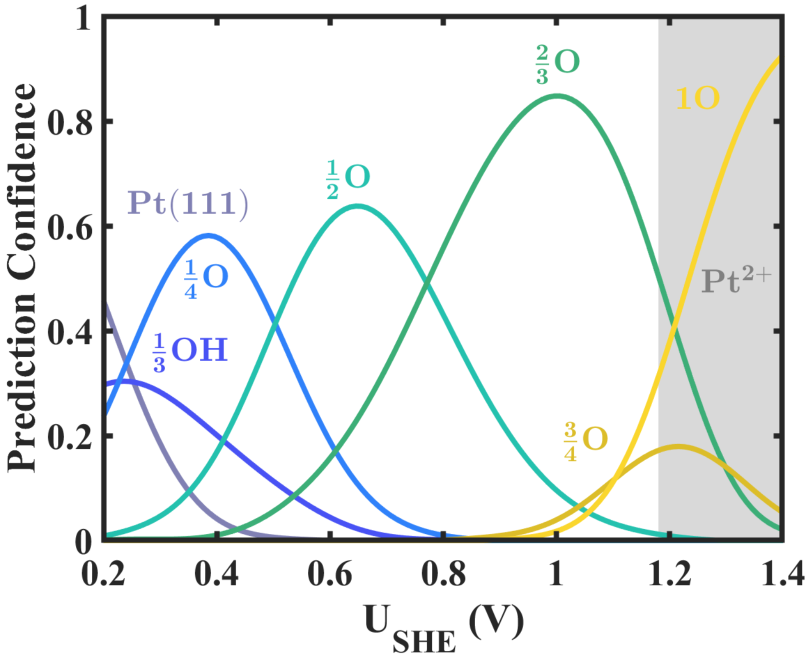


Figure S10: Prediction confidence of surface states considered on Pt(111) at pH of 7.

# 9 Other Supplementary Figures

## 9.1 Pt(100)

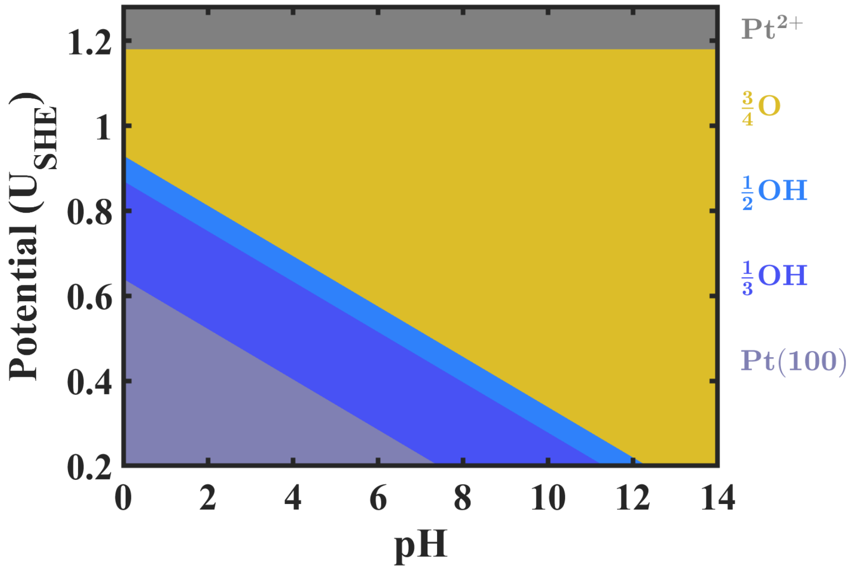


Figure S11: Surface Pourbaix diagram of Pt(100) derived from the best-fit BEEF-vdW XC-functional.

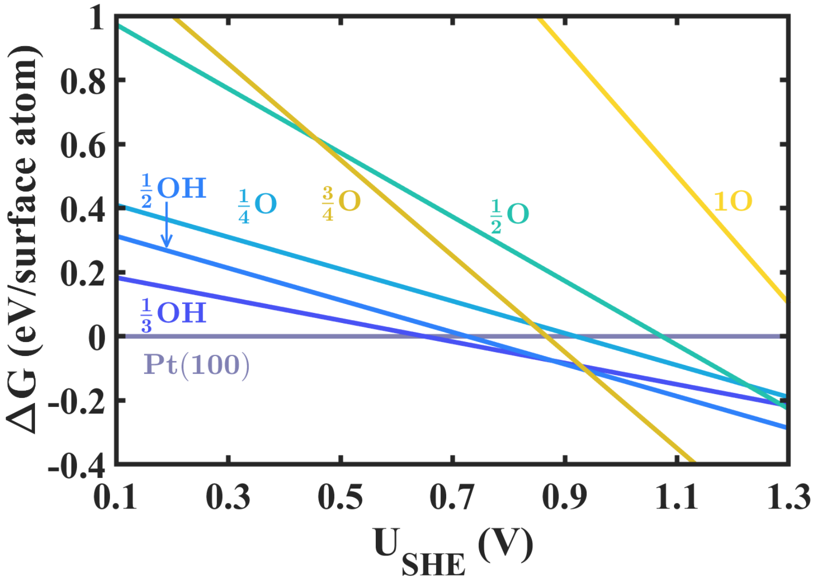


Figure S12: Stability of surface phases considered on Pt(100) in terms of free energy at pH=0. Bold lines are calculated from the best-fit BEEF-vdW functional.

## 9.2 Pd(111)

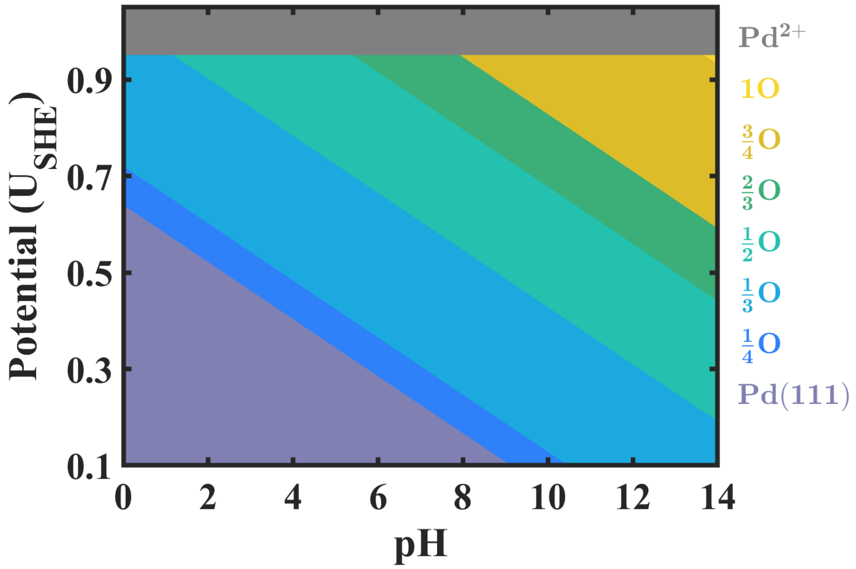


Figure S13: Surface Pourbaix diagram of Pd(111) derived from the best-fit BEEF-vdW XC-functional.

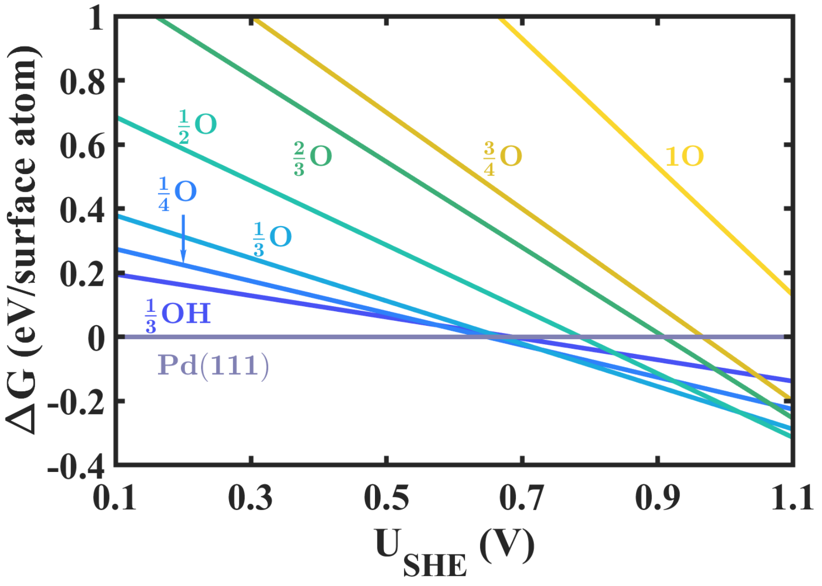


Figure S14: Stability of surface phases considered on Pd(111) in terms of free energy at pH=0. Bold lines are calculated from the best-fit BEEF-vdW functional.

## 9.3 Ir(111)

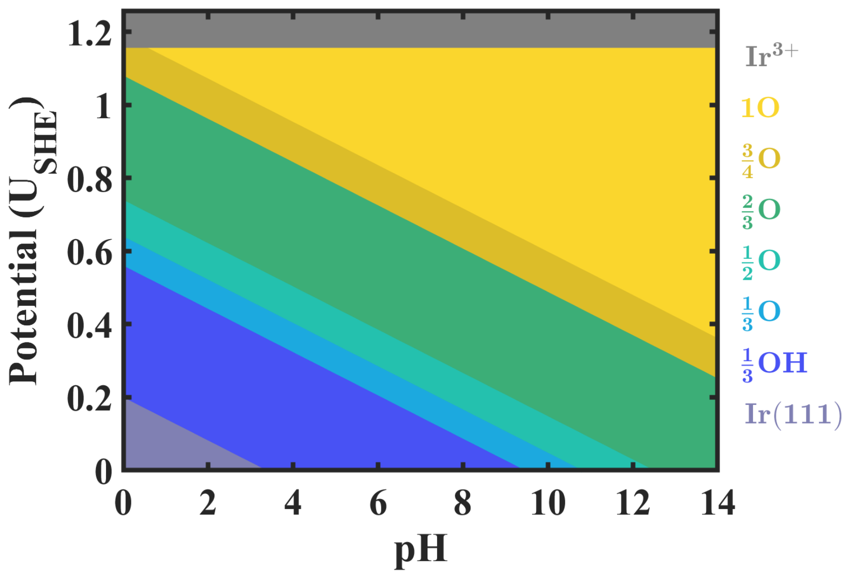


Figure S15: Surface Pourbaix diagram of Ir(111) derived from the best-fit BEEF-vdW XC-functional.

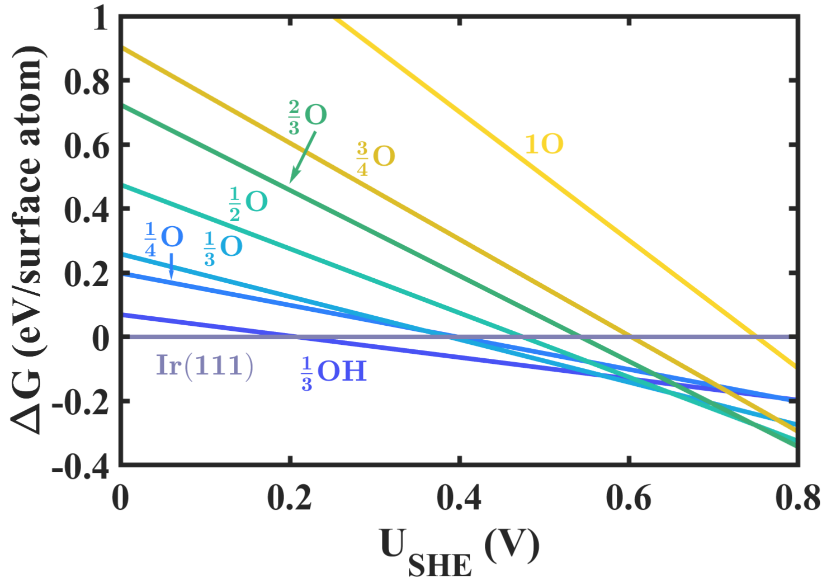


Figure S16: Stability of surface phases considered on Ir(111) in terms of free energy at pH=0. Bold lines are calculated from the best-fit BEEF-vdW functional.

## 9.4 Rh(111)

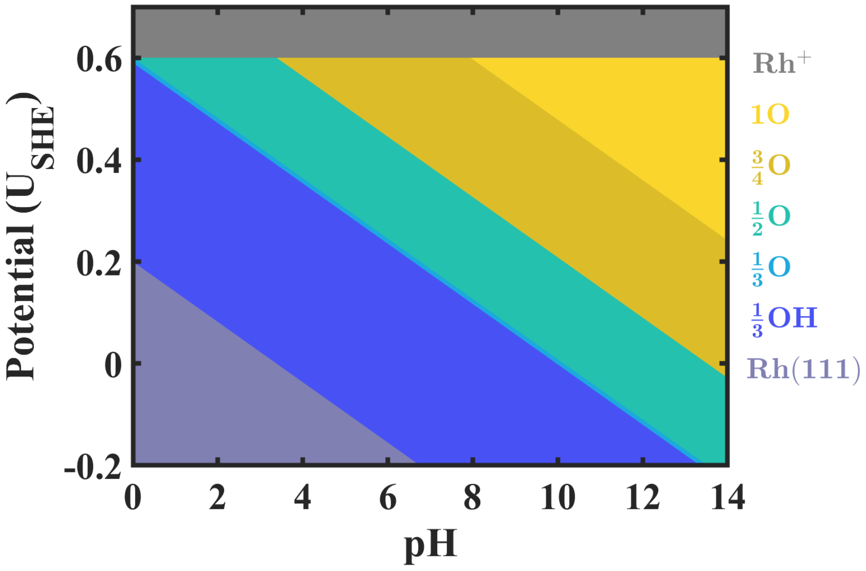


Figure S17: Surface Pourbaix diagram of Rh(111) derived from the best-fit BEEF-vdW XC-functional.

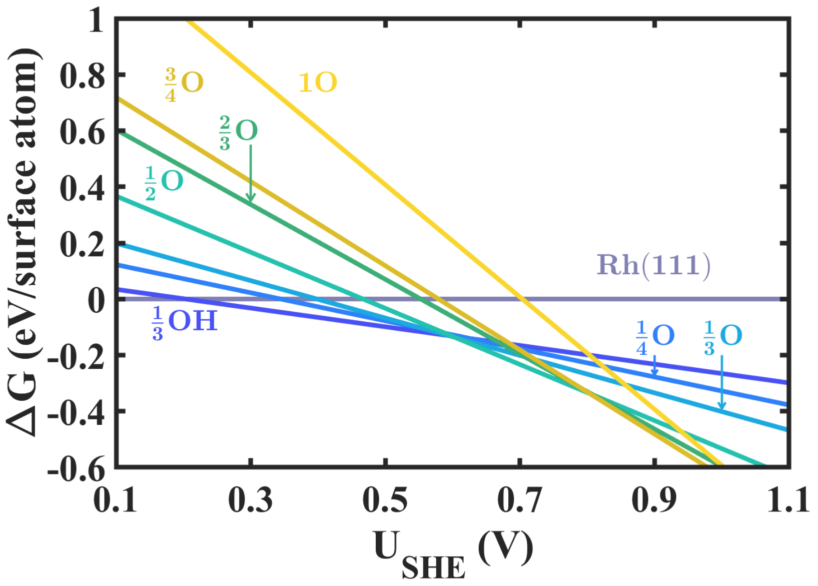


Figure S18: Stability of surface phases considered on Rh(111) in terms of free energy at pH=0. Bold lines are calculated from the best-fit BEEF-vdW functional.

## 9.5 Ru(0001)

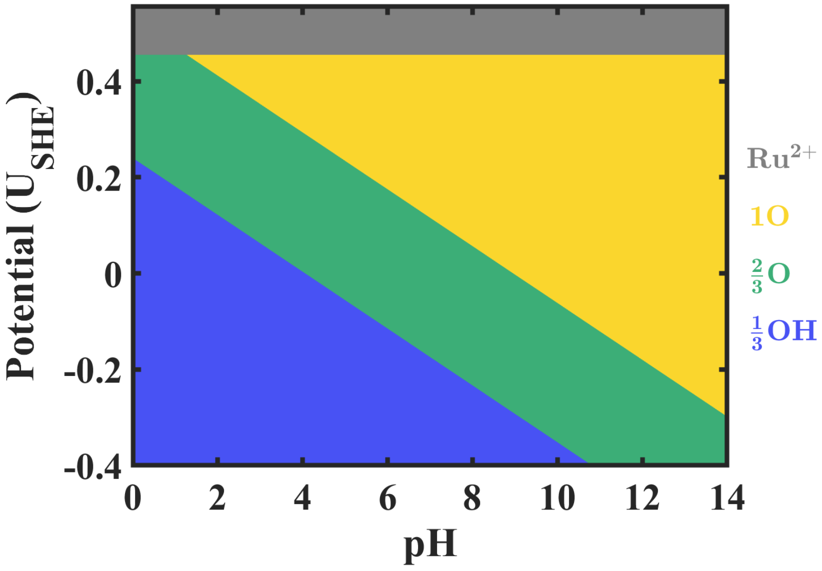


Figure S19: Surface Pourbaix diagram of Ru(0001) derived from the best-fit BEEF-vdW XC-functional.

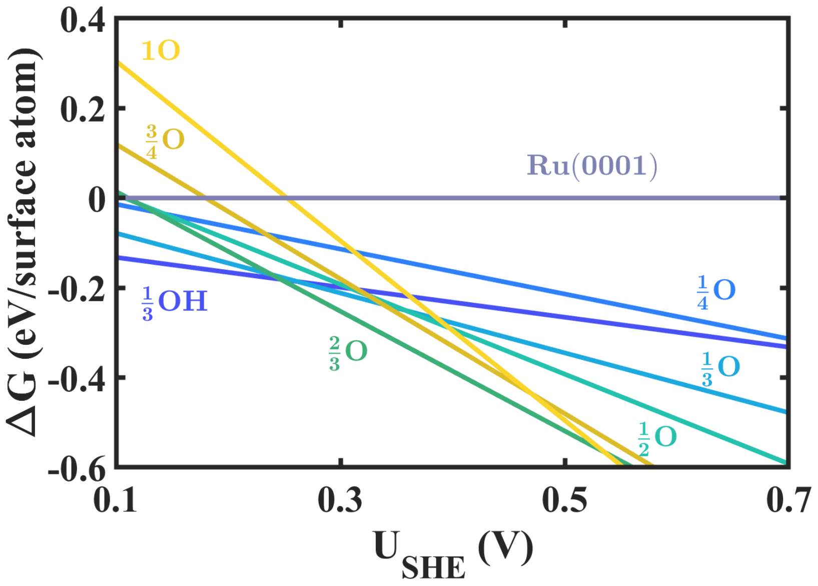


Figure S20: Stability of surface phases considered on Ru(0001) in terms of free energy at pH=0. Bold lines are calculated from the best-fit BEEF-vdW functional.

# References


(1) Blöchl, P. E. Projector augmented-wave method. *Phys. Rev. B* **1994**, *50*, 17953.

(2) Kresse, G.; Joubert, D. From ultrasoft pseudopotentials to the projector augmented-wave method. *Phys. Rev. B* **1999**, *59*, 1758–1775.

(3) Mortensen, J. J.; Hansen, L. B.; Jacobsen, K. W. Real-space grid implementation of the projector augmented wave method. *Phys. Rev. B* **2005**, *71*, 035109.

(4) Monkhorst, H. J.; Pack, J. D. Special points for Brillouin-zone integrations. *Phys. Rev. B* **1976**, *13*, 5188.

(5) Larsen, A. H. et al. The atomic simulation environment a Python library for working with atoms. *J. Phys. Condens. Matter* **2017**, *29*, 273002.

(6) Wellendorff, J.; Lundgaard, K. T.; Møgelhøj, A.; Petzold, V.; Landis, D. D.; Nørskov, J. K.; Bligaard, T.; Jacobsen, K. W. Density functionals for surface science: Exchange-correlation model development with Bayesian error estimation. *Phys. Rev. B* **2012**, *85*, 235149.

(7) Medford, A. J.; Wellendorff, J.; Vojvodic, A.; Studt, F.; Abild-Pedersen, F.; Jacobsen, K. W.; Bligaard, T.; Nørskov, J. K. Assessing the reliability of calculated catalytic ammonia synthesis rates. *Science* **2014**, *345*, 197–200.

(8) Deshpande, S.; Kitchin, J. R.; Viswanathan, V. Quantifying Uncertainty in Activity Volcano Relationships for Oxygen Reduction Reaction. *ACS Catal.* **2016**, *6*, 5251–5259.

(9) Krishnamurthy, D.; Sumaria, V.; Viswanathan, V. Maximal predictability approach for identifying the right descriptors for electrocatalytic reactions. *J. Phys. Chem. Lett.*

(10) Houchins, G.; Viswanathan, V. Quantifying confidence in density functional theory predictions of magnetic ground states. *Phys. Rev. B* **2017**, *96*, 134426.

(11) Ahmad, Z.; Viswanathan, V. Quantification of uncertainty in first-principles predicted mechanical properties of solids: Application to solid ion conductors. *Phys. Rev. B* **2016**, *94*, 064105.

(12) Atkins, P. W. *Physical Chemistry*, 6th ed.; Oxford University Press, 1998.

(13) Kandoi, S.; Gokhale, A.; Grabow, L.; Dumesic, J.; Mavrikakis, M. Why Au and Cu are more selective than Pt for preferential oxidation of CO at low temperature. *Catal. Lett.* **2004**, *93*, 93–100.
